# Supplementary material for: Determination of Calibration Parameters of Cantilevers of Arbitrary Shape by Finite Elements Analysis
Source: arXiv:2010.12451 ancillary file (2021-09-07)
Supplement: Supplementary file 1 [file supplementary_info.pdf]

*Supplementary Material*

# Determination of Calibration Parameters of Cantilevers of Arbitrary Shape by Finite Elements Analysis

Jorge Rodriguez Ramos*, Felix Rico

AFFILIATIONS

Aix-Marseille University, INSERM, CNRS, LAI.

*Author to whom correspondence should be addressed: jorge.r.ramos@outlook.com

**Supporting figures and tables**

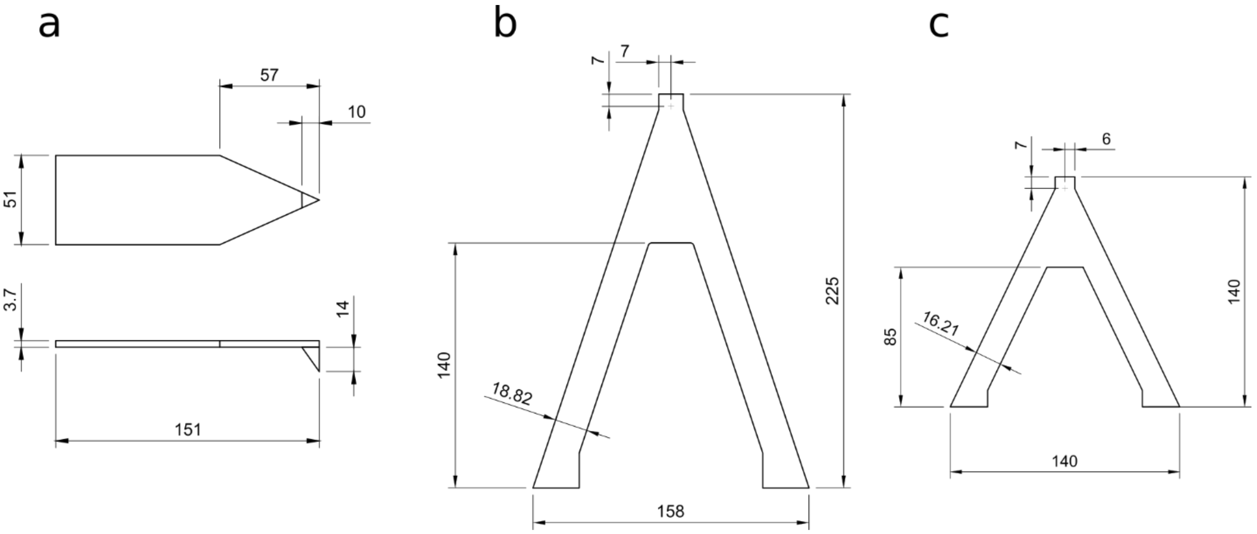


Figure S1. Relevant dimensions of AC160TS (a), MLCT-BIO-DC-D (b) and MLCT-BIO-DC-E (c) cantilevers.

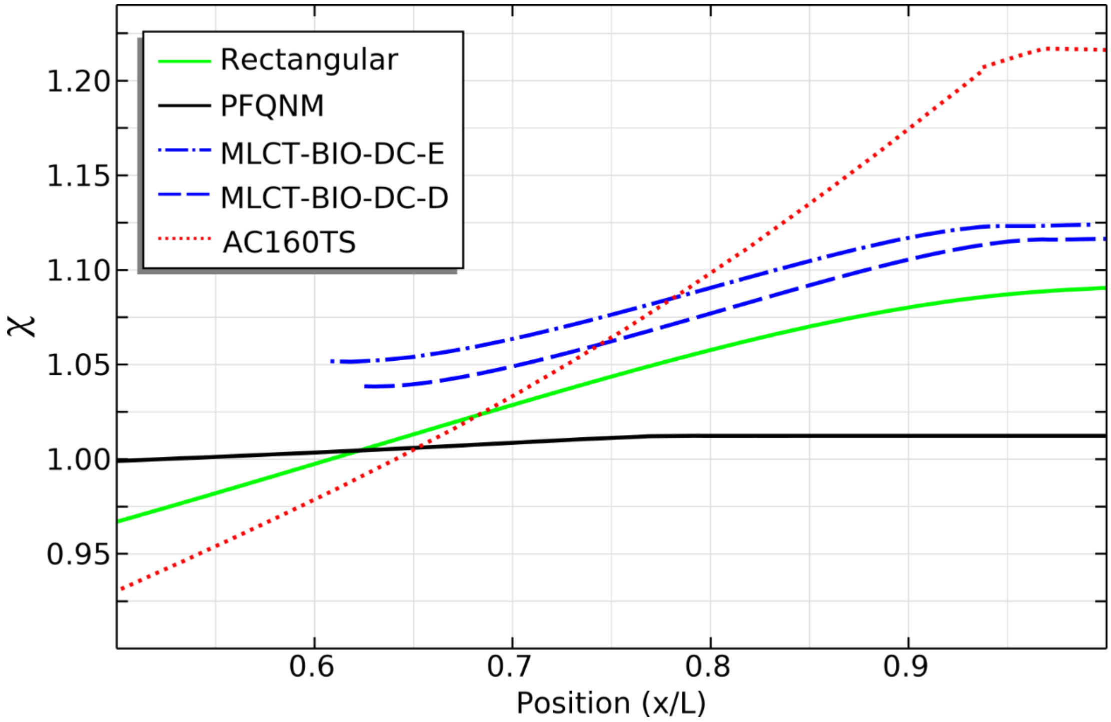


Figure S2. Correction factor $\chi$ for the cantilever geometries modelled.

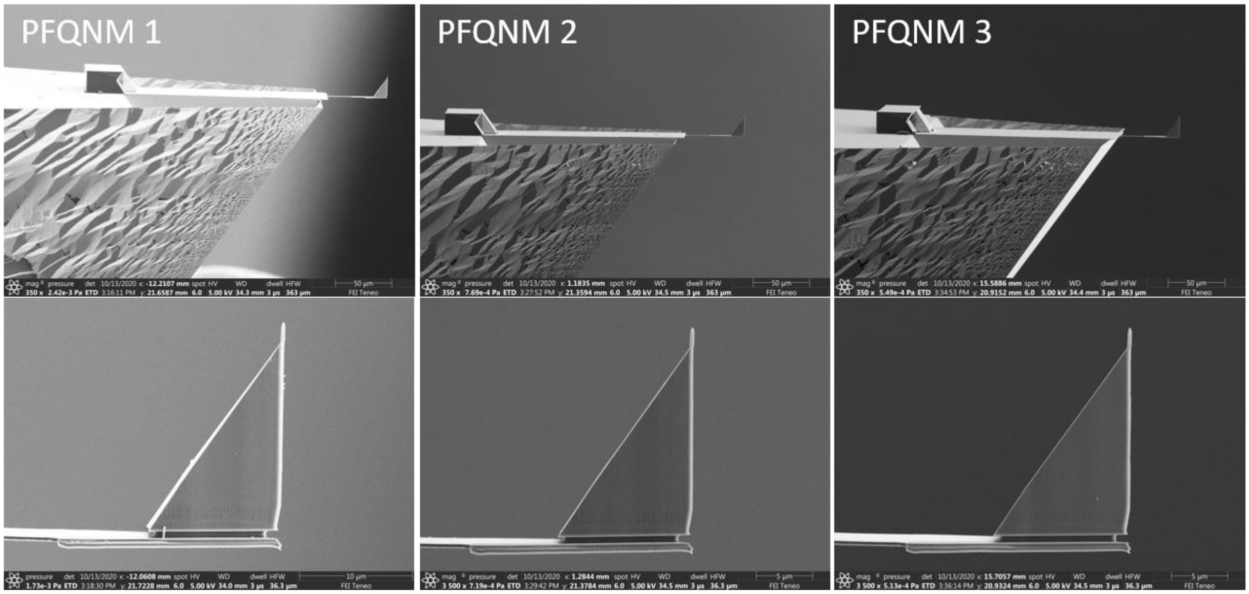


Figure S3. SEM images of the PFQNM cantilever used in this work. The micrographs were recorded after the experiments. The magnification is 350x and 3500x for the upper and lower rows, respectively.

Table S1. Influence of the reflecting gold layer on PFQNM calibration parameters.

| Au coating | $\frac{m_{\mathrm{tip}}}{m_c}$ | $\frac{m_{\mathrm{eff}}}{m_c}$ | $f_1$ (kHz) | $k_c$ (mN/m) | $k_1$ (mN/m) | $\beta$ | $\chi$ | $\frac{\beta}{\chi^2}$ |
|---|---|---|---|---|---|---|---|---|
| None | 0.75 | 0.63 | 42.3 | 57.8 | 57.9 | 0.9979 | 1.012 | 0.974 |
| 25 nm | 0.66 | 0.58 | 43.3 | 63.9 | 64.1 | 0.9970 | 1.015 | 0.968 |
| 50 nm | 0.58 | 0.55 | 44.6 | 71.8 | 72.1 | 0.9963 | 1.016 | 0.964 |
